# Supplementary material for: Multivariate Business Process Representation Learning utilizing Gramian Angular Fields and Convolutional Neural Networks
Source: arXiv:2106.08027 source file (2021-06-15)
Supplement: Supplementary file 1 [file appendix.tex]

\section{Appendix}

\section{Problem Statement}
The research gap in business process representation learning\cite{Weerdt_2018} is tackled and the next step towards better models that are able to solve complex tasks on business process data. In order to generate a generic feature vector from arbitrary business process perspectives, process executions are encoded as gramian angular fields\cite{Wang_2014} and processed with a combination of CNN and feed-forward neural network. Using a proper learning strategy, the models learns to generate a feature vector that contains all relevant information captured in the data which can be used for next step prediction, outcome prediction, clustering, anomaly detection and other problems. We demonstrate the models ability to represent process executions on different tasks, i.e. outcome prediction, clustering and anomaly detection (and maybe next step prediction).\\
The justification of recurrent neural networks for these predictive process analytics is given by sequential nature of process data and the ability of these model to process such data\cite{Evermann_2017}. However, what is often not considered in depth is the multivariate and multi-scalar nature of business process data in comparison to other sequential data like natural language %(this comparison is e.g. drawn by \cite{Evermann_2016}).
When modelling only one perspective of a business process, e.g. the control-flow, process data is very similar to natural language and prediction the next activity in a trace is very similar to predicting the next word in a sentence. However, when the next activity is not only depending on previous activities but on a another attribute, e.g. the costs, the comparison is limp. In real-life business process data, decisions are often depending on contextual attributes rather than solely on sequence of the previous actions/activities. We will demonstrate this on a small example.

\subsection{Example}
For predicting the next activity in an ongoing case it is important to have access to all the information necessary at this point in the process. However, for anomaly detection one must find deviations in the interaction between several attributes.

\begin{figure}[!h]
    \centering
    \includegraphics[width=0.8\textwidth]{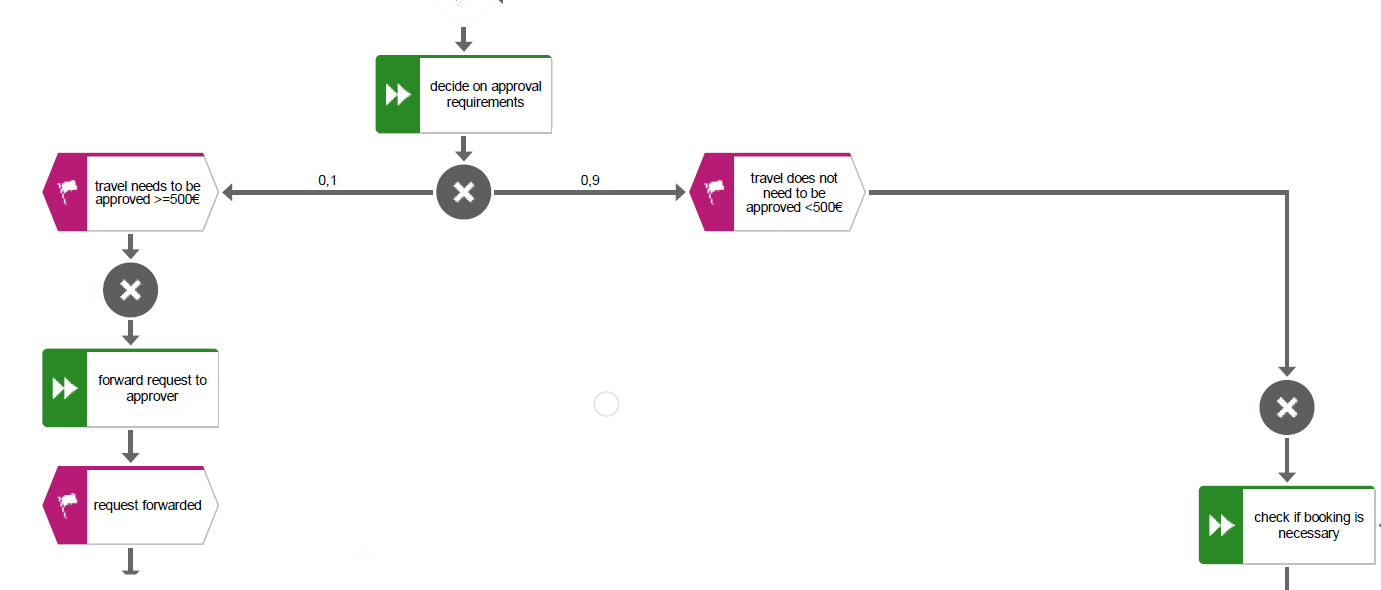}
    \caption{Snippet of the MobIS Travel Process}
    \label{fig:MobIS}
\end{figure}

Figure \ref{fig:MobIS} shows as excerpt of a travel management process. At this point, the process has two different path how to continue depending solely on the costs. In order to predict the next activity in a case after "decide on approval requirements", one must know the cost. If they are above or equal to 500 the next activity is "forward request to approver", if they are below 500 the next activity is "check if booking is necessary". In case of anomaly detection given a trace with costs above 500, one has to check the costs, the activities executed and their order as well the resource who executed each activity and sometimes also their timestamps. For this simple example, this task is already very complex and can only be solved when all relevant information is processed jointly.

\newpage

\section{Development}
Only for documentation purposes!

\subsubsection{Experiments}
\paragraph{Pre-training}
As GAfs are very different to natural images, we tried to pre-train MVCNN, especially CNN1, on a variant classification task. That is, given a case c, predict its variant. This helps a lot in later tasks. Accuracy is much higher from the beginning on if using a pre-trained CNN1.\\
Current setting: All variants with at least 5 cases. 140 classes, 100\% acc.\\
At least 2 cases: 300 classes, 98.9\% accuracy.

\paragraph{Mulit-task pre-training}
Pre-trained on MobIS to predict the next activity, next resource, next type, timestamp and cost.\\
Same accuracy as trained on next activity only.

\paragraph{colored vs. greyscale images}
In order to get rid of the very slow coloring function of matplotlib, we directly used the output of the GAF transformation and scaled them to (0, 255). This makes the computation much fast but decreases the accuracy not notable. 

\paragraph{Max-pooling vs. con-cat layer}
The original MVCNN uses a max-pooling layer between CNN1 and CNN2. While it works very well for renders of 3D models, it does not work well using event log data. Therefore, we tested a concat layer, that concatenates the output of CNN1 from perspective 1..n. If using the concat layer, CNN2 has the same size, i.e. \#num\_perspectives * feature\_size. This gives much higher accuracy's in the next-step-prediction task.

\paragraph{Attention}
Implement Attention mechanism after CNN1 (pooling) to make CNN2 attentive to certain pattern.

\paragraph{Results NSP MobIS}
88-92\% accuracy. Same as LSTM. Many splits in the process are not predictable as no information is in the data. LSTM often learns the distribution of these decisions (can be compared to the distribution of the simluation) while MPPN uses the whole data.\\
However, one split after "decide on approval requirements" depends on the costs. While LSTM learns the distribution, MPPN learns this dependency from the data. All other descicions are not predictable.

\subsection{Issue}

\begin{itemize}
    \item Slow to train
    \item Too many attributes decrease accuracy when doing representation learning. Training loss decreases but validation loss increases.
\end{itemize}

\subsubsection{Things to work on}
\begin{itemize}
    \item GAF size: Padding required or not?
    \item CNN1: Size, dimension...
    \item Which feature pooling? Concatenation or max-pooling, ...
    \item Hyperparameter tuning (NUmber neurons per layer, learning rate, activation function...)
    \item Concatenate all GAFs to one.
    \item Masking
    \item Attention
    \item GAF colored or greyscale
    \item Long sequences
\end{itemize}
